# Supplementary material for: Decidability of Querying First-Order Theories via Countermodels of Finite Width
Source: arXiv:2304.06348 source file (2025-04-21)
Supplement: Supplementary file 1 [file treewidth-hyperclique-proof.tex]

\begin{proof}
Let $T = (V,E)$ be a tree-decomposition of $\inst$ witnessing that $\inst$ has a treewidth of $k$. Then, the countability of $\inst$ implies the countability (and thus, countable degree) of $T$. Therefore, by repeatedly introducing $E$-neighboring copies of nodes, $T$ can be transformed into a full (directed) binary tree $T'=(V',E',\termset)$ with $V'= \{0,1\}^*$, $E'= \{(s,s0), (s,s1) \mid s\in\{0,1\}^*\}$, and $\termset:V'\to 2^{\adom{\inst}}$, which inherits all tree decomposition properties from $T$. The moderate reformulation using the $\termset$ function is necessary due to the introduction of node copies containing identical sets of terms.

Let $\fcn{slot}: \adom{\inst} \to \{0,\ldots,k\}$ be a function that satisfies $\fcn{slot}(t_1)\neq \fcn{slot}(t_2)$ for any $t_1\neq t_2$ with $\{t_1,t_2\} \subseteq \termset(s)$ for some $s\in V'$; note that the existence of such a function is guaranteed by the treewidth bound of $T'$ inherited from $T$. For a tuple $\vt = (t_{1}, \ldots, t_{n})$ of terms, we define $\fcn{slot}(\vt) = (\fcn{slot}(t_{1}), \ldots, \fcn{slot}(t_{n}))$. Moreover, for each domain element $t\in \adom{\inst}$ let $\fcn{pivot}(t)$ denote the node $s \in V'$ with $t \in \termset(s)$ that is closest to the root of $T'$. Also, for each tuple $\vt\in\adom{\inst}^{m}$ with $1 \le m\le \arity{\Sigma}$, let $\fcn{pivot}(\vt)$ denote the node $s\in V'$ that is closest to the root of $T'$ with $t \in \termset(s)$ for each term $t$ occurring in the tuple $\vt$.

For each atom $\rpred(\pi[\vt_1\concat\vt_2]) \in \inst$ and permutation $\pi$ on $\{ 1, \ldots \arity{\rpred} \}$, one of the following three statements must hold for $T'$:

\begin{itemize}
	\item $\fcn{pivot}(\vt_1) = \fcn{pivot}(\vt_2)$, denoted $\vt_1 \approx \vt_2$,
	\item $\fcn{pivot}(\vt_1)$ is an ancestor of $\fcn{pivot}(\vt_2)$, denoted $\vt_1 \prec \vt_2$,
	\item $\fcn{pivot}(\vt_2)$ is an ancestor of $\fcn{pivot}(\vt_1)$, denoted $\vt_2 \prec \vt_1$.
\end{itemize}
 where the the empty tuple is $\prec \vt$ for every nonempty tuple $\vt$. Furthermore, we use $\vec{\downarrow}$ to denote a tuple consisting solely of some number of $\downarrow$ symbols. If we wish to be specific about the number of elements in a tuple $\vec{\downarrow}$, we write $\vec{\downarrow}_{m}$ to indicate that the corresponding tuple contains $m$ occurrences of $\downarrow$.

	For each $1 \le m\le \arity{\Sigma}$, let the finite set $\cols_{m}$ consist of the tuples $(j_1, \ldots, j_m, S)$ with $0 \le j_1, \ldots, j_m \le k$ and $S$ be a subset of
	$$
	\{ (\rpred(\vec{\downarrow}_{m} \hspace{-1ex}{\concat}  \vec{i}), \pi) \mid \rpred \in \Sigma_{>m}, \vec{i}\in\{ 0, \ldots, k\}^{\arity{\rpred} - m}, \text{ and } \pi \text{ is a permutation on } \{ 1, \ldots, \arity{\rpred} \} \}.
	$$
	We set $\cols$ to be the union of the (finitely many) $\cols_{m}$, and provide a description of the process of transforming~$T'$ into an $(\cols,\mathrm{Cnst})$–well-decorated infinite binary tree representing $\inst$. For a node $s$ of $T'$, we define $\fcn{tf}(s)$ as follows:

\begin{itemize}
\item Take a fresh node $v$, decorate it with $\oplus$, and set its two children to be $\fcn{tf}(s0)$ and $\fcn{tf}(s1)$ with $s0$ and $s1$ the two children of $s$ in $T'$. Set $v$ to be the {\em current root} of the transformation.
\item Next, for each $t \in \adom{\inst}$ with $\fcn{pivot}(t)=s$, which we assume are in ascending order by $\fcn{slot}(t)$ (there are at most $k+1$ of such terms), do the following:
    \begin{enumerate}
    \item Take a fresh node $v'$, decorate it with $\oplus$, and make the current root $v$ its left child and let its right child be a fresh node $u$ decorated with $\precol_{\origcol \to (j, S)}$ and having a fresh left child node $z$ (i.e. $z$ is set as the left child of $u$), which is decorated by $t$ if $t \in \mathrm{Cnst}$, or $\const{*}$ otherwise, and where $j = \fcn{slot}(t)$ and $S$ contains:
        \begin{itemize}
%        \item[$\circ$] \textcolor{gray}{all $\rpred(\downarrow)$ with $\rpred(t) \in \inst$ and all $\rpred(\downarrow,\downarrow)$ with $\rpred(t,t) \in \inst$, } \textcolor{thomas}{Should be subsumed by the next entry and case $m=2$ later on, by the assumption that the empty tuple of terms is always a ``pivotal ancestor'' of every tuple.}
        \item[$\circ$] all $(\rpred(\downarrow,\vec{i}), \pi)$ with $\rpred(\pi[t\concat\vt']) \in \inst$ for some $\vt' \in \adom{\inst}^{\arity{\rpred} - 1}$ with $\fcn{slot}(\vt')=\vec{i}$ and where either $\vt'\prec t$, or if $\vt'\approx t$, then $\min\{i \ | \ i \in \vec{i}\}>j$.
        \end{itemize}
    \item Build a chain $P$ of nodes decorated with $\pcadd$ and $\precol$ predicates to reflect the following set of operations:
        \begin{itemize}
        \item[$\circ$] for every unary colorset containing $(j,S)$, for which $S$ contains some $\rpred(\downarrow)$, perform %$\fcadd_{(j,S), \rpred}$ and then 
        $\frecol_{(j,S)\to \{ (j,S \setminus \{\rpred(\downarrow)\}) \} \cup \{ \rpred \}}$,
        \item[$\circ$] for any two colors $(j,S)$ and $(\vec{i},S')$ where $m  =\arity{\vec{i}, S'}$, for which $S'$ contains some $(\rpred(\vec{\downarrow}_m,j), \pi)$, perform $\fcadd_{(\vec{i},S')(j,S), \rpred}^{\pi}$ and immediately afterward perform $\frecol_{(\vec{i},S')\to(\vec{i},S' \setminus \{(\rpred(\vec{\downarrow},j), \pi)\})}$.
        \end{itemize}
    \item Set the current root to be the highest node of $P$ and set $v'$ to be the child of the lowest node of $P$.
    \item Denote the current node by $v^{1}$.
    \end{enumerate}
\item Next, assume the current node to be $v^{m-1}$. Go through all $\vt \in \adom{\inst}^{m}$ with $\fcn{pivot}(\vt)=s$, which we assume are in ascending order induced lexicographically by $\fcn{slot}(\vt)$ (there are at most $(k+1)^{m}$ of such terms) and build the following chain $P$:
\begin{enumerate}
	\item Start building the chain $P$ as a chain of nodes decorated with $\pcadd$ reflecting for every $(\vec{j}, S)\in \cols_{m-1}$ and $(j, S')\in \cols_1$ the operations $\fcadd_{(\vec{j}, S)(j, S'), (\vec{j}\concat j, S'')}$ where $\vec{j} = \fcn{slot}(t_1, \ldots, t_{m-1})$, $j = \fcn{slot}(t_m)$ and $S''$ contains all $(\rpred(\vec{\downarrow}_m\! \concat \ \vec{i}), \pi)$ such that $\rpred(\pi[\vt\concat\vt'])\in\inst$ for some $\vt'$ from $\adom{\inst}$ with $\fcn{slot}(\vt') = \vec{i}$ and where either $\vt'\prec \vt$, or  if $\vt'\approx \vt$, then $\min{\vec{i}} > \max{\vec{j}}$.
	\item Extend the chain $P$ by adding nodes decorated with $\pcadd$ and $\precol$ predicates to reflect the following set of operations:
	\begin{itemize}
		\item[$\circ$] for every colorset of $< m$-ary colors containing $(\vec{j},S)$, for which $S$ contains some $\rpred(\vec{\downarrow})$, perform %$\fcadd_{(j,S), \rpred}$ and then 
		$\frecol_{(\vec{j},S)\to \{ (\vec{j},S \setminus \{\rpred(\downarrow)\}) \} \cup \{ \rpred \}}$,
		\item[$\circ$] for any two colors $(\vec{j},S)$ and $(\vec{i},S')$, for which $S'$ contains some $(\rpred(\vec{\downarrow}_{\length{\vec{i}}}\concat\vec{j}), \pi)$, perform $\fcadd_{(\vec{i},S')(\vec{j},S), \rpred}^{\pi}$ and immediately afterward $\frecol_{(\vec{i},S')\to(\vec{i},S' \setminus \{(\rpred(\vec{\downarrow}_{\length{\vec{i}}}\concat\vec{j}), \pi)\})}$.
	\end{itemize}
	\item Set the current root to be the highest node of $P$ and set $v^{m-1}$ to be the child of the lowest node of $P$.
	\item Denote the current node by $v^{m}$.
\end{enumerate}
\end{itemize}

To obtain $\fcn{tf}(s)$, take the resulting decorated tree and extend the resulting tree to an infinite binary tree by adding missing elements and decorating them with $\pred{Void}$.

Finally, take the root $\varepsilon$ of $T'$ and obtain $\fcn{tf}(\varepsilon)$ based on the above procedure. After, add nodes decorated with $\pcadd_\rpred^{\pi}$ above the root of $\fcn{tf}(\varepsilon)$ (in any order), where $\pi : \emptyset \to \emptyset$ is the empty permutation and $\rpred \in \Sigma$ is a nullary predicate with $\rpred \in \inst$. Once again, add in any missing nodes to create an infinite binary tree and decorate such nodes with $\pred{Void}$. The resulting $(\cols,\mathrm{Cnst})$-well-decorated tree represents $\inst$.
\end{proof}
